# Supplementary material for: Renormalization of a Contact Interaction on a Lattice
Source: arXiv:1912.04425 source file (2020-01-16)
Supplement: Supplementary file 1 [file appendix.tex]

\section{Misc}

We can put the derivation of the counter terms etc. in appendices.

Do we want to put tables?  Make numerical data directly available?  We should be good, reproducible scientists.

\input{section/appendix/dispersion-coefficients}
\input{section/appendix/counterterm/spherical}
\input{section/appendix/counterterm/cartesian}
\input{section/appendix/counterterm/dispersion}
\input{section/appendix/two-d}
\section{Continuum extrapolation}\label{sec:continuum}

\begin{figure}[ht!]
\center
\input{figure/a1g-state-overlap.pgf}
\caption{A1g state ovelap\label{fig:a1g-state-overlap}}
\end{figure}

\begin{figure}[ht!]
\center
\input{figure/continuum-spectrum_a-inv_+0.0_zeta_spherical_projector_a1g_n-eigs_200.pgf}
\caption{A1g state ovelap\label{fig:a1g-state-overlap}}
\end{figure}
